# Supplementary material for: Long-Horizon Visual Planning with Goal-Conditioned Hierarchical Predictors
Source: arXiv:2006.13205 source file (2020-11-27)
Supplement: Supplementary file 1 [file supplement.tex]

\documentclass{article}

\usepackage[nonatbib,final]{neurips_2020}

\usepackage[utf8]{inputenc} %
\usepackage[T1]{fontenc}    %
\usepackage{hyperref}       %
\usepackage{url}            %
\usepackage{booktabs}       %
\usepackage{amsfonts}       %
\usepackage{nicefrac}       %
\usepackage{microtype}
\usepackage{graphicx}
\usepackage{subfigure}
\usepackage[svgnames]{xcolor}
\usepackage{algorithm2e}
\usepackage{algorithm}
\usepackage[noend]{algorithmic}

\usepackage{hyperref}

\usepackage{color}

\usepackage{varwidth}
\usepackage{xspace}

\input{math_commands.tex}

\newcommand{\todo}[1]{ \textcolor{red}{\bf #1}}

\definecolor{clr}{cmyk}{0, 0.7808, 0.4429, 0.1412}

\renewcommand{\todo}[1]{}

\usepackage{mathtools}
\usepackage{amsmath,amssymb}
\usepackage{bm}
\usepackage{siunitx}
\usepackage{wrapfig}
\sisetup{output-exponent-marker=\ensuremath{\mathrm{e}}}
\sisetup{detect-weight=true, detect-family=true}

\makeatletter
\def\blfootnote{\xdef\@thefnmark{}\@footnotetext}
\makeatother

\usepackage[numbers]{natbib}
\bibliographystyle{plainnat}

\title{Supplementary Material: \\ 
Long-Horizon Visual Planning with GCPs}

\begin{document}
\maketitle

\appendix
\input{sections/appendix.tex}
\bibliography{bibref_definitions_long,bibtex}

\end{document}
